# Supplementary material for: Hard No-Box Adversarial Attack on Skeleton-Based Human Action Recognition with Skeleton-Motion-Informed Gradient
Source: arXiv:2308.05681 source file (2023-08-18)
Supplement: Supplementary file 1 [file supplement.pdf]

# Hard No-Box Adversarial Attack on Skeleton-Based Human Action Recognition with Skeleton-Motion-Informed Gradient – Supplementary Material

Zhengzhi Lu[1,2 †] He Wang[3] Ziyi Chang[1] Guoan Yang[2] Hubert P. H. Shum[1 ‡]
[1]Durham University, UK [2]Xi'an Jiaotong University, China [3]University College London, UK
lu947867114@stu.xjtu.edu.cn he_wang@ucl.ac.uk ziyi.chang@durham.ac.uk
gayang@mail.xjtu.edu.cn hubert.shum@durham.ac.uk

In this document, we first show extra experimental results for hard no-box attacks and the data fitting of time-varying autoregressive models. Then, we give the details of SMI-FGSM and the transfer-based black-box attack. Furthermore, we describe the data augmentation approaches used in contrastive learning. Finally, we show the attack results of hard no-box attacks against a defense method.

## 1. Visual Comparisons

We demonstrate more static poses of adversarial samples under different attack strategies in no-box attacks. These samples are conducted on the NTU60 datasets and the perturbation budget $\epsilon$ is 0.006. The visual comparisons are shown in Figure 1. It is obvious that SMI gradient-based attack methods improve the imperceptibility compared with their baselines. We provide more examples in the supplementary video.

## 2. The Number of Cluster Centers for Negative Samples

The selection of negative samples is crucial in our hard no-box attacks. Hence, we utilize the K-means clustering method to obtain proper negative samples. In this part, we study how the no-box fooling rate varies with different numbers of cluster centers in the K-means. The number of cluster centers in K-means is set as 120, 100, 80, and 60, respectively. I-FGSM [2] is adopted to generate hard no-box adversarial samples on the NTU60. The fooling rates under different numbers of cluster centers are reported in Table 1. All samples in the test dataset are used for clustering. The attack with 120 cluster centers achieves the best results when attacking MS-G3D and AS-GCN. The fooling rate of 60 cluster centers is similar to 120 and even outperforms in js-AGCN. We speculate this might be because the NTU60 dataset is divided into 60 classes.

† This work was conducted during the visit to the Durham University.
‡ Corresponding Author

| Victims | 120 | 100 | 80 | 60 |
|---|---|---|---|---|
| js-AGCN | 27.84% | 27.62% | 26.89% | **28.02%** |
| MS-G3D | **11.13**% | 10.43% | 10.70% | 11.03% |
| AS-GCN | **14.08**% | 13.65% | 13.90% | 14.02% |

Table 1. The fooling rate of the different numbers of cluster centers in no-box attacks with $\epsilon = 0.01$.

## 3. Trading-Off Sample Size and Fooling Rate in Cluster

We utilize all the samples in the test dataset for K-means clustering in hard no-box attacks. However, it is possible to trade-off between the number of samples used in clustering and the fooling rate. To reduce the calculation burden, not all the samples are necessary for clustering. We conduct the no-box attack results on the NTU60 with different numbers of cluster samples, i.e. 100%, 75%, 50%, and 25% of the dataset. We employ I-FGSM to produce no-box adversarial samples and show the fooling rates in Table 2. The number of cluster centers is set as 120. Using fewer samples for clustering slightly reduces the fooling rate but gives a better trade-off.

| Victims | 100% | 75% | 50% | 25% |
|---|---|---|---|---|
| js-AGCN | **27.84**% | 27.22% | 27.05% | 26.51% |
| MS-G3D | **11.13**% | 10.83% | 10.85% | 10.80% |
| AS-GCN | **14.08**% | 13.45% | 13.92% | 13.43% |

Table 2. The no-box fooling rate of different numbers of samples used in clustering, $\epsilon = 0.01$.

## 4. Other Comparisons

### 4.1. Selecting Negative Samples

Positive samples indicate boundary of same class while negative ones indicate high-density areas of other classes. As shown in Table 3, our ablation study shows selecting negative ones avoids misleading perturbations.

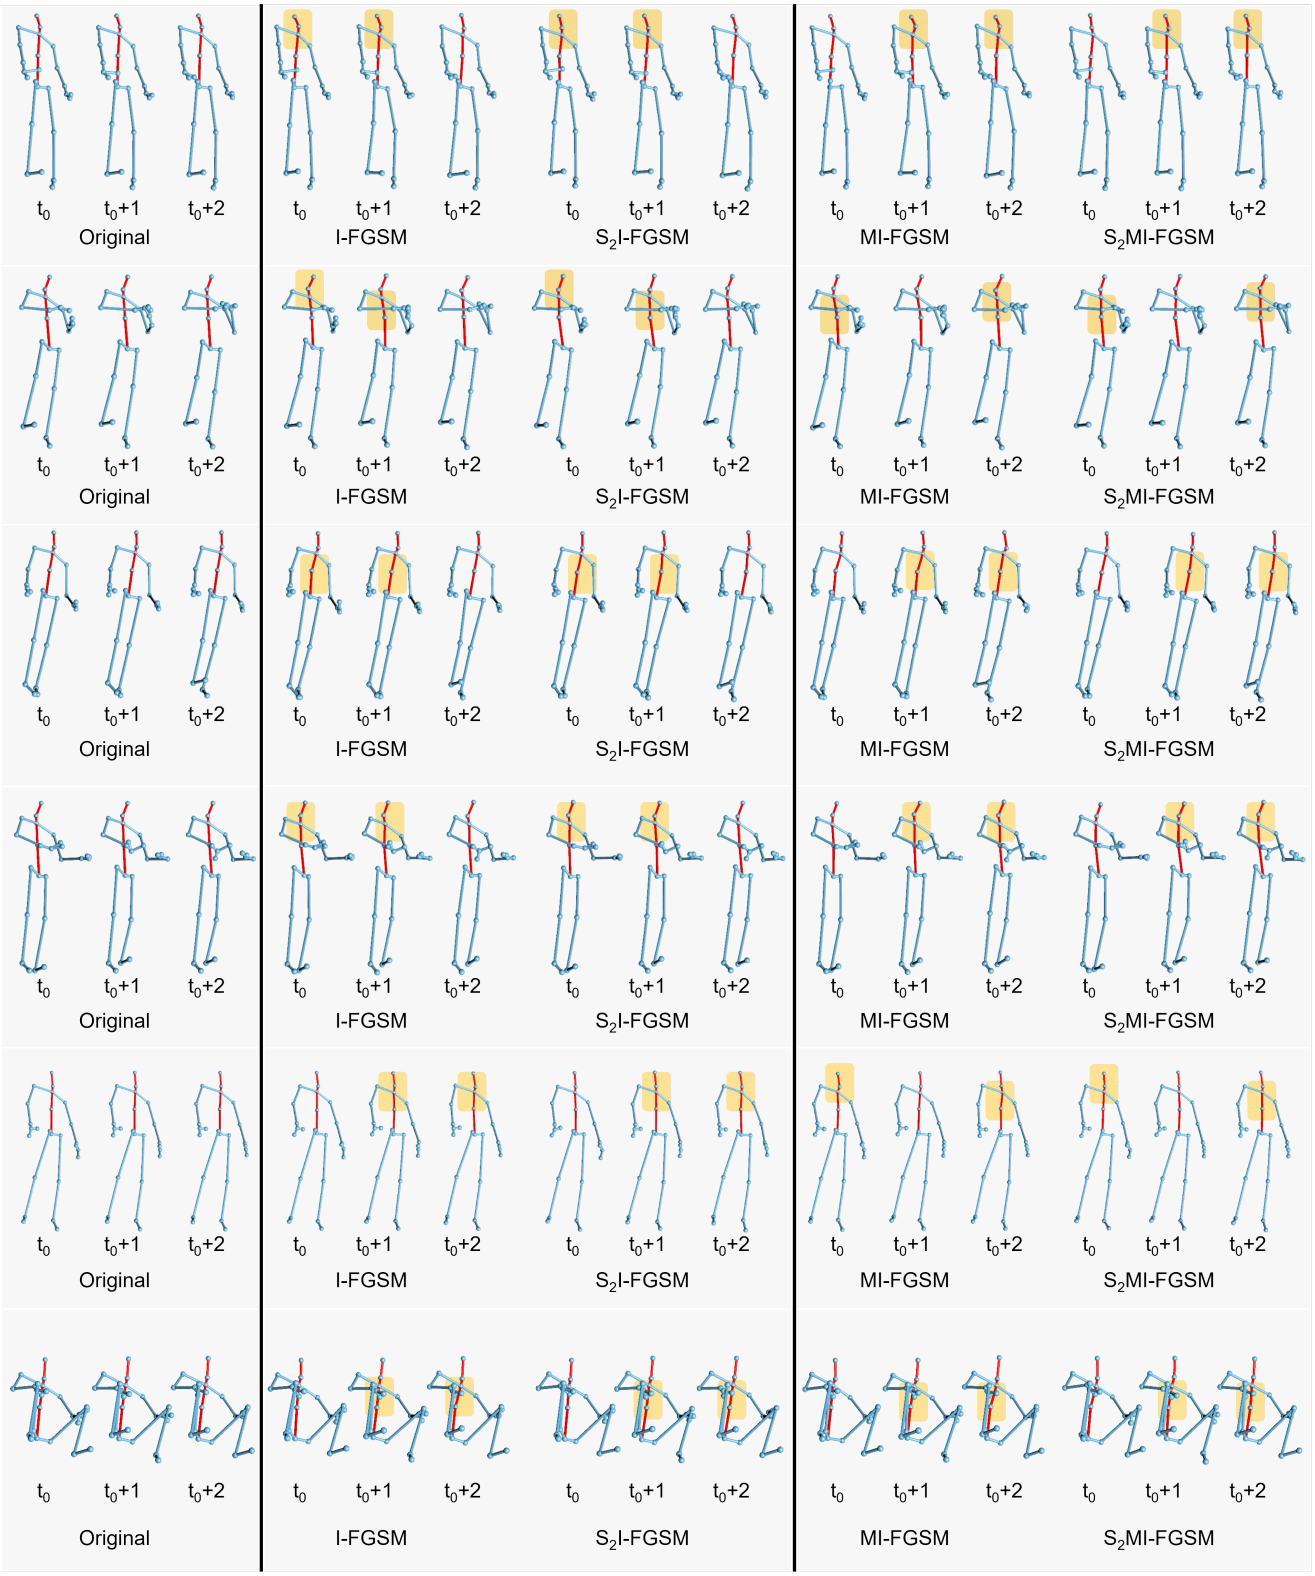


Figure 1. Visual comparisons between attack strategies in no-box attacks ($\epsilon$=0.006) with key visual differences highlighted.

| Victims | w/o | w |
|---|---|---|
| js-AGCN | 31.5% | **36.6%** |
| MS-G3D | 11.1% | **14.1%** |

Table 3. The fooling rate of $S_2$MI-FGSM against js-AGCN and MS-G3D without or with selection of nagative samples in no-box attacks on NTU60 with $\epsilon = 0.01$.

### 4.2. Adaptating Previous Methods to Motions

Our hard no-box setting is the strictest when compared with no-box, black-box and white-box settings. Particularly, previous no-box methods uses different, looser settings where labels are usually required. On the contrary, our hard no-box setting is stricter and does not require labels. Moreover, our proposed method explicitly considers motion dynamics while previous no-box methods are usually proposed for images without any dynamics-related consideration. Nonetheless, we still adapt a no-box method [3] to the motion data to validate our dynamics consideration. Table 4 shows simple adaptation of previous methods to motion data leads to worse fooling rates even if more knowledge is used in their methods. [3] struggles to capture skeleton dynamics but our method with SMI gradient is effective.

| Victims | [3] Method | Our Method |
|---|---|---|
| js-AGCN | 11.64% | **26.05%** |
| MS-G3D | 4.92% | **9.55%** |

Table 4. The fooling rate of adapting [3] to motions and our method against js-AGCN and MS-G3D on NTU60 with $\epsilon = 0.01$.

### 4.3. Training with Training Samples Other Than Testing Ones

Our proposed method does not necessarily require testing samples that are used for attacking, and allows to be trained on other samples. Table 5 shows the fooling rates when our method is trained on test or other samples (samples in the training set).

| Victims | Testing Samples | Other Samples |
|---|---|---|
| js-AGCN | 30.87% | **35.30%** |
| MS-G3D | 11.69% | **12.98%** |

Table 5. The fooling rate of $S_2$MI-FGSM being trained on testing samples or other samples against js-AGCN and MS-G3D on NTU60 with $\epsilon = 0.01$.

### 4.4. Training with Half Dataset

Our method does not rely on full dataset for both training and attacking. We report results in Table 6. The distribution shift in non-overlap samples for training and attacking may lead to this slight difference.

| Victims | Full Set | Half Set |
|---|---|---|
| js-AGCN | **9.96%** | 8.78% |
| MS-G3D | **11.69%** | 9.30% |

Table 6. The fooling rate of $S_2$MI-FGSM being trained on full or half training dataset against js-AGCN and MS-G3D on NTU60 with $\epsilon = 0.01$.

## 5. Data Fitting Performance of Time-varying Autoregressive

In order to estimate SMI gradient, we employ time-varying autoregressive (TV-AR) to model the dynamic relationship in skeletal sequences. This section demonstrates the skeletal data fitting results of TV-AR(1) and TV-AR(2) models. Our TV-AR models constrain the mapping of the dynamics to a specific situation, i.e. they assume that each degree of freedom (DOF) of skeletal data is independent of the others. The fitting curves are shown in Figure 2. Both the TV-AR(1) and TV-AR(2) successfully model the skeletal sequences, and TV-AR(1) gets better fitting results.

## 6. The Detailed Algorithm of SMI-FGSM

In this section, we provide the algorithm of SMI-FGSM. It is obtained by integrating the momentum term of gradients into each iteration of SI-FGSM. The whole process is shown in the Algorithm 1.

**Algorithm 1** $S_1$MI-FGSM and $S_2$MI-FGSM

**Input:** An encoder $k$ with loss function $J$; a skeletal sequence samples $S$; the size of attack step $\alpha$; the number of iterations $I$; the budget of perturbation $\epsilon$; the weight decay factor $\mu$.

**Output:** An adversarial example $\hat{S}$ with $\|\hat{S} - S\|_p < \epsilon$.

Initialization: $\hat{S}^0 = S$, $(g^0)_{d1} = 0$, $(g^0)_{d2} = 0$;

Fitting $S$ with TV-AR model to obtain the time-varying parameters $\beta_t$;

**for** $i = 0$ to $I - 1$ **do**

  Inputting $\hat{S}^i$ to $k$;

  Using loss function $J$ to obtain the raw gradient $\nabla J(\hat{S}^i)$;

  Calculating the SMI gradient $(\nabla J(\hat{S}^i))_{d1}$ with Eq.9, or $(\nabla J(\hat{S}^i))_{d2}$ with Eq.10 using $\beta_t$ and $\nabla J(\hat{S}^i)$;

  Updating $(g^{i+1})_{d1}$ or $(g^{i+1})_{d2}$ by accumulating the velocity vector in the gradient direction as

$$(g^{i+1})_{d1} = \mu \cdot (g^i)_{d1} + \frac{(\nabla J(\hat{S}^i))_{d1}}{\left\|(\nabla J(\hat{S}^i))_{d1}\right\|_1}, or$$
$$(g^{i+1})_{d2} = \mu \cdot (g^i)_{d2} + \frac{(\nabla J(\hat{S}^i))_{d2}}{\left\|(\nabla J(\hat{S}^i))_{d2}\right\|_1}; \tag{1}$$

  Updating $\hat{S}^{i+1}$ by applying the sign gradient as

$$\hat{S}^{i+1} = \hat{S}^i + \alpha \cdot \text{sign}\left((g^{i+1})_{d1}\right), or$$
$$\hat{S}^{i+1} = \hat{S}^i + \alpha \cdot \text{sign}\left((g^{i+1})_{d2}\right); \tag{2}$$

**end for**

**return** $\hat{S} = \hat{S}^I$

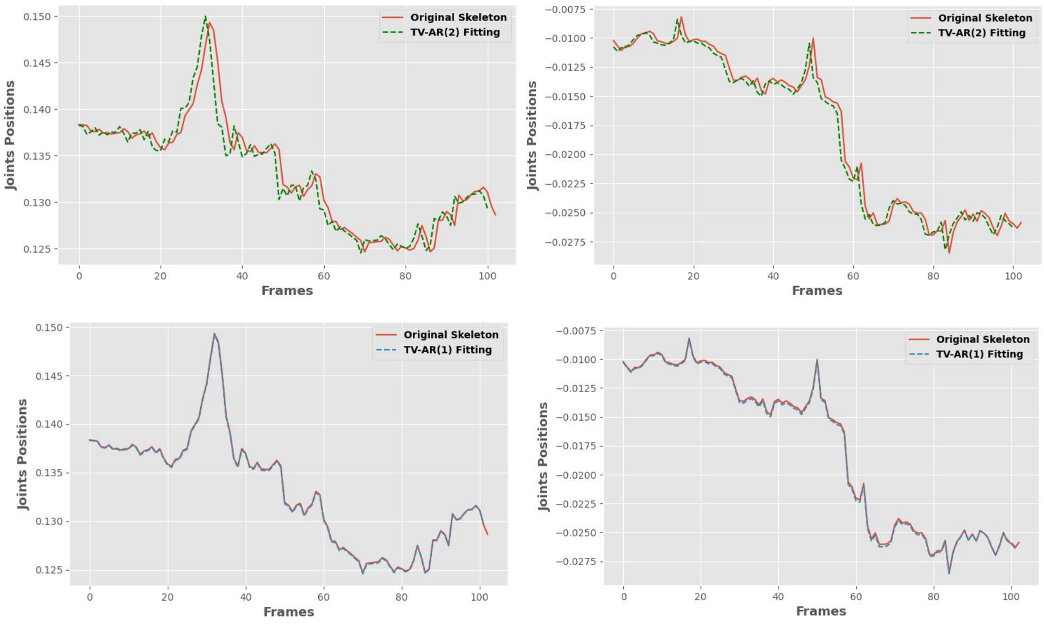


Figure 2. Skeletal data fitting of TV-AR model. Upper is TV-AR(2) model, and lower is TV-AR(1) model.

## 7. The Details of Transfer-Based Black-Box Attacks

We employ SMART [6] as the baseline for the transfer-based black-box attack. SMART is a white-box attacker which utilizes classification loss and perceptual loss to generate adversarial samples. In our experimental settings, the attack step size $\alpha$ of SMART is set as 0.005, and the maximum iteration number is 400. In the transfer-based black-box attack, due to SMART having the full knowledge of the surrogate models, we adopt an early stop strategy following its original settings. This means SMART ends the iterative attack when it succeeds in the white-box attack to ensure the best imperceptibility. Therefore, not all the samples are iterated for the 400 epochs. This is a crucial distinction between the no-box attack and the transfer-based black-box attack.

## 8. Skeleton Augmentations for Contrastive Learning

In this section, we detail the skeleton augmentation methods used in training the latent manifold for the hard no-box attack through contrastive learning (CL). These augmentations can be divided into temporal augmentations and spatial augmentations. We combine these two methods to create positive samples for CL. The spatial augmentations contain pose transformation and joint jittering. The temporal augmentations are temporal crop and resize. We assume that $S$ is the input skeletal sequence consisting of body joints $L$ in $T$ frames.

**Pose Transformation** We utilize pose transformation to obtain the augmented samples that retain the same pose as the input but vary in viewpoint and distance to the camera. The 3D shearing is adopted to the skeletal sequence $S$ at each frame for pose transformation:

$$D_{\text{pose}}(S) = S \cdot \begin{bmatrix} 1 & r_{01} & r_{02} \\ r_{10} & 1 & r_{12} \\ r_{20} & r_{21} & 1 \end{bmatrix}, \tag{3}$$

where $r$ is randomly selected from a uniform distribution $[-1, 1]$. We show some samples of pose transformation in Figure 3.

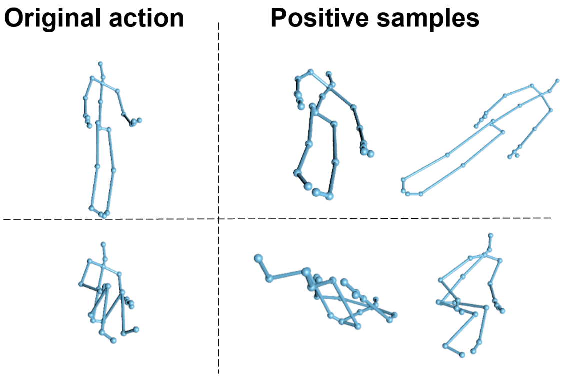


Figure 3. Pose transformation augmented samples.

**Joint Jittering** To enhance the performance of the no-box attack, we aim to train a data manifold that is robust to the

noise and random changes. Hence, we employ joint jittering where the selected joints are randomly moved into irregular positions. The augmentations can be defined as:

$$D_{\text{joint}}(S) = S[:, l] \cdot \begin{bmatrix} r_{00} & r_{01} & r_{02} \\ r_{10} & r_{11} & r_{12} \\ r_{20} & r_{21} & r_{22} \end{bmatrix}, \quad (4)$$

where $r$ is randomly selected from a uniform distribution $[-1, 1]$ and $l$ is a subset of joints randomly chosen for each motion. The same transformation matrix is applied to each frame in one motion. Examples are shown in Figure 4.

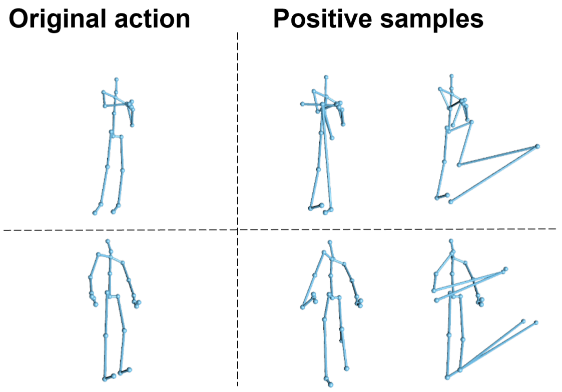


Figure 4. Joint jittering augmented samples.

**Temporal crop and resize** Temporal relationship is critical to skeletal-related downstream tasks. Therefore, we change the speed, and starting and ending points in the original samples to create positive pairs. The temporal crop and resize can be expressed as:

$$D_{\text{Temporal}}(S) = \text{Interpolate}\left(S\left[R_{\text{start}} : R_{\text{end}}\right]\right), \quad (5)$$

where $R_{\text{start}}$ and $R_{\text{end}}$ are the randomly selected starting and ending points. We first create a new sub-sequence $(S\left[R_{\text{start}} : R_{\text{end}}\right])$, and then re-sample it to a fixed length. The interpolation helps to get the samples varying in speeds. Figure 5 shows the examples of temporal crop and resize,

We combine the above spatial and temporal augmentations to obtain positive samples for CL. We first apply the temporal crop and resize to the inputs $S$. Then we randomly choose the spatial augmentation from the pose transformation and the joint jittering and adopt it to the temporal augmented samples.

## 9. Attack Results Against Defense Method

We employ randomized smoothing [1] for defense to test our post-defense performance. The robustness of randomized smoothing largely depends on a defense budget $\sigma$, which is the magnitude of the noise added during robust

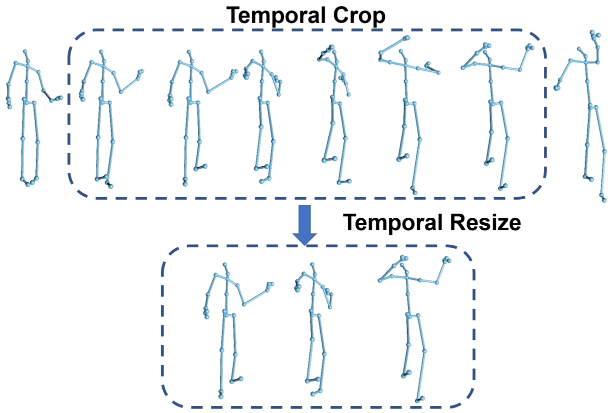


Figure 5. Temporal crop and resize.

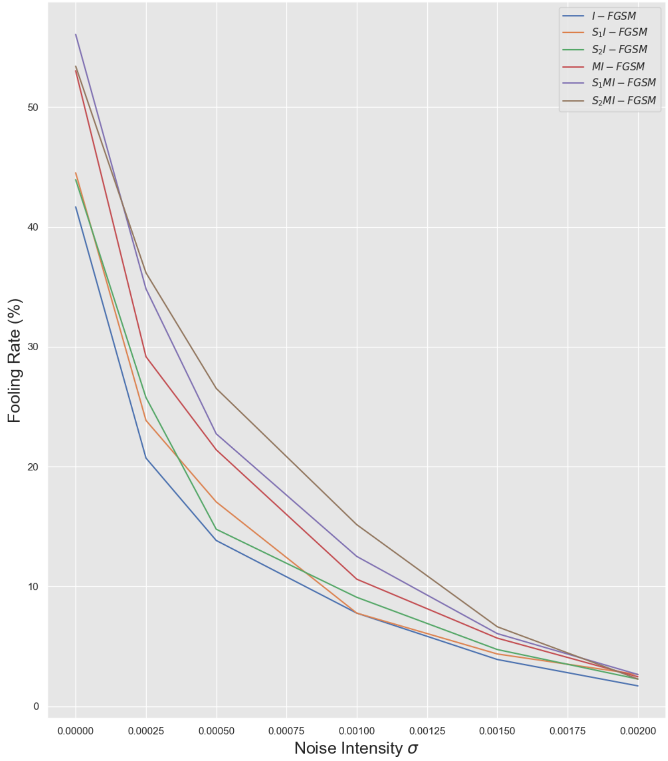


Figure 6. Fooling rates of attack methods under different noise intensities.

training. We test different $\sigma$ values to improve its robustness. Here, we choose MS-G3D [4] as the victim model as it is one of the latest classifiers and HDM05 as the dataset [5]. After training, we launch our hard no-box attacks using different attack strategies. Fooling rates of these strategies under different noise magnitudes are shown in Figure 6. With the improvement of the robustness of the victim model, naturally the fooling rate of all the attack methods has decreased, but we notice that SMI gradient still boosts the performance compared with the raw gradient. Admit-

tedly, hard-no box attacks are not as effective as other attack methods, especially post-defense, but it is only because our method has extremely limited knowledge about the data and the victim model, compared with the settings of existing methods. We argue that the hard no-box attack is the least restrictive attack setting so far, which itself is a contribution.

## References


[1] Jeremy Cohen, Elan Rosenfeld, and Zico Kolter. Certified adversarial robustness via randomized smoothing. In *international conference on machine learning*, pages 1310–1320. PMLR, 2019.

[2] Alexey Kurakin, Ian J Goodfellow, and Samy Bengio. *Adversarial examples in the physical world*, pages 99–112. Chapman and Hall/CRC, 2018.

[3] Qizhang Li, Yiwen Guo, and Hao Chen. Practical no-box adversarial attacks against dnns, 2020.

[4] Ziyu Liu, Hongwen Zhang, Zhenghao Chen, Zhiyong Wang, and Wanli Ouyang. Disentangling and unifying graph convolutions for skeleton-based action recognition. In *Proceedings of the IEEE/CVF conference on computer vision and pattern recognition*, pages 143–152, 2020.

[5] Meinard Müller, Tido Röder, Michael Clausen, Bernhard Eberhardt, Björn Krüger, and Andreas Weber. Mocap database hdm05. *Institut für Informatik II, Universität Bonn*, 2(7), 2007.

[6] He Wang, Feixiang He, Zhexi Peng, Tianjia Shao, Yong-Liang Yang, Kun Zhou, and David Hogg. Understanding the robustness of skeleton-based action recognition under adversarial attack. In *Proceedings of the IEEE/CVF Conference on Computer Vision and Pattern Recognition*, pages 14656–14665, 2021.
